# Supplementary material for: Percolation and electrical conduction in random systems of curved linear objects on a plane: computer simulations along with a mean-field approach
Source: arXiv:2301.12795 ancillary file (2023-01-30)
Supplement: Supplementary file 1 [file arcs2023SM.pdf]

## Supplemental Material.
# Percolation and electrical conduction in random systems of curved linear objects on a plane: computer simulations along with a mean-field approach

Yuri Yu. Tarasevich,* Andrei V. Eserkepov,† and Irina V. Vodolazskaya‡
*Laboratory of Mathematical Modeling, Astrakhan State University, Astrakhan, 414056, Russia*

This Supplemental Material presents the derivation of the average number of contacts between arcs.

## I. PROBLEM STATEMENT, GENERAL REMARKS AND NOTATION

*a. A problem.* There are two circles of radius $r$. Each circle has an arc based on the central angle $\varphi$ ($\varphi \in [0; 2\pi]$). The distance between the centers of the circles is equal to $x$ ($0 \leqslant x \leqslant 2r$). The locations of the arcs on the circles are equiprobable. Find conditions under which the arcs have one and two points of intersection.

*b. Technical details.* Let the origin of coordinates coincide with the center of the first circle, and let the abscissa axis be directed so that it passes through the center of the second circle. Let the ray directed from the center of the first circle to the middle of the arc on this circle has an angle with the abscissa axis $\alpha_1$. Let the ray directed from the center of the second circle to the middle of the arc on this circle has an angle with the abscissa axis $\alpha_2$. It is assumed that $\alpha_1, \alpha_2 \in [-\pi; \pi]$.

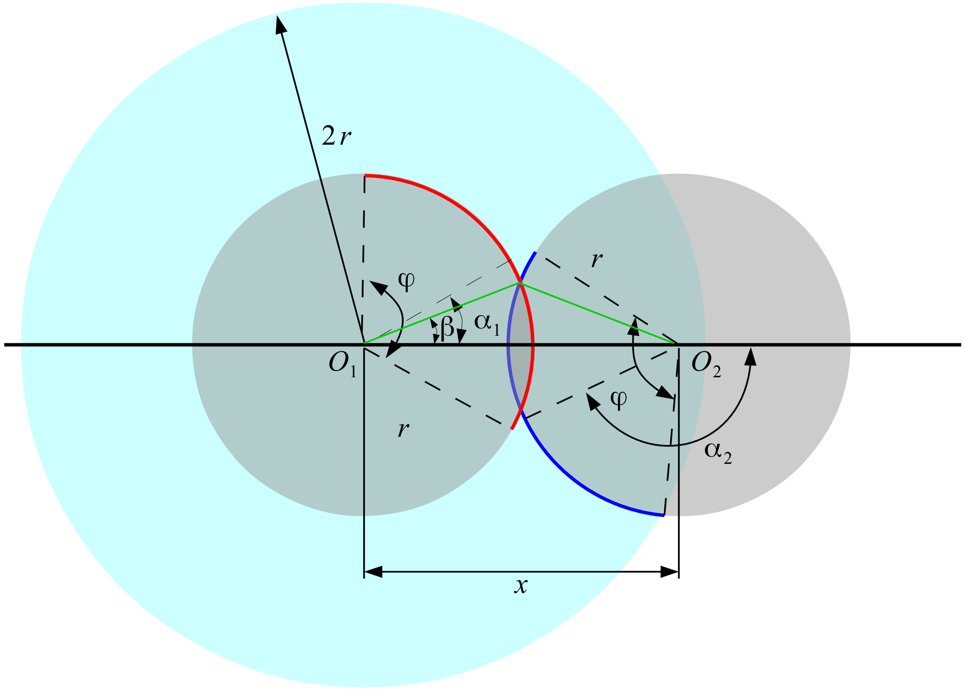


FIG. 1. Sketch to explain the derivation of formulas

The angular coordinates of the intersection points of the circles relative to the center of the first circle are

$$\beta_{1,2} = \pm\beta(x), \quad \text{where} \quad \beta(x) = \arccos \frac{x}{2r}.$$

* Corresponding author: tarasevich@asu.edu.ru
† dantealigjery49@gmail.com
‡ vodolazskaya_agu@mail.ru

Notice, that

$$\max \beta(x) = \beta(0) = \frac{\pi}{2}.$$

The angular coordinates of the arc ends relative to the center of the first circle are

$$\alpha_1 \pm \frac{\varphi}{2}.$$

The intersection point of the circles lies on an arc belonging to the first circle if

$$\alpha_1 - \frac{\varphi}{2} < \arccos \frac{x}{2r} < \alpha_1 + \frac{\varphi}{2},$$

$$\alpha_1 - \frac{\varphi}{2} < -\arccos \frac{x}{2r} < \alpha_1 + \frac{\varphi}{2}.$$

*c. Probability notation.* The subscript indicates the number of the circle. The probability without a subscript refers to the number of intersections of the arcs. The superscript in brackets is the number of intersection points of the circles that belong to the considered arc. Probability without a superscript indicates the probability of arc intersections (the number of intersection points does not matter).

## II. THE FIXED DISTANCE BETWEEN CIRCLE CENTERS

### A. The case of small arcs

If $\varphi < 2\beta(x)$, then only one point of intersecting circles can lie on an arc, and arcs cannot intersect twice.

$$P_1^{(2)}(x) = P_2^{(2)}(x) = P^{(2)}(x) = 0, \quad \text{if} \quad x < 2r \cos \frac{\varphi}{2}.$$

The probability that either of the two intersection points of the circles lies on the marked arc of the first circle is

$$P_1^{(1)}(x) = \frac{\varphi}{\pi}.$$

The probability that the same intersection point of the circles lies on the marked arc of the second circle is

$$P_2^{(1)}(x) = \frac{\varphi}{2\pi}.$$

The probability that the marked arcs intersect once is

$$P(x) = P^{(1)}(x) = P_1^{(1)}(x) P_2^{(1)}(x) = \frac{\varphi^2}{2\pi^2}, \quad \text{if} \quad x < 2r \cos \frac{\varphi}{2}.$$

### B. The case of large arcs

If $\varphi > 2\pi - 2\beta(x)$, at least one of the intersection points of the circles has to be located on the arc. Both intersection points of the circles lie on the marked arc of the first circle with probability

$$P_1^{(2)}(x) = \frac{\varphi}{\pi} - 1.$$

Similarly, both intersection points of the circles lie on the marked arc of the second circle with probability

$$P_2^{(2)}(x) = \frac{\varphi}{\pi} - 1.$$

The probability that the marked arcs intersect twice is

$$P^{(2)}(x) = P_1^{(2)}(x) P_2^{(2)}(x) = \left(\frac{\varphi}{\pi} - 1\right)^2.$$

The probability that the arcs do not intersect. Let the marked arc of the first circle not contain the upper intersection point. The probability of this event is

$$P_1^* = \frac{2\pi - \varphi}{2\pi}.$$

Let the marked arc of the second circle not contain the lower intersection point. The probability of this event is

$$P_2^* = \frac{2\pi - \varphi}{2\pi}.$$

The probability of simultaneous execution of these events is equal to

$$P_1^* P_2^* = \left(\frac{2\pi - \varphi}{2\pi}\right)^2.$$

The probability that the arcs do not intersect is

$$P^{(0)} = 2P_1^* P_2^* = 2\left(\frac{2\pi - \varphi}{2\pi}\right)^2.$$

Probability of intersecting arcs

$$P(x) = 1 - P^{(0)} = 1 - 2\left(\frac{2\pi - \varphi}{2\pi}\right)^2 = \frac{2\varphi}{\pi} - \frac{\varphi^2}{2\pi^2} - 1.$$

Obviously,

$$P^{(0)} + P^{(1)} + P^{(2)} = 1.$$

Then

$$P^{(1)} = \frac{4\varphi}{\pi} - \frac{3\varphi^2}{2\pi^2} - 2.$$

### C. The case of intermediate arcs

If $\varphi + 2\beta(x) < 2\pi$, then the arc can have two points of intersection of circles, one or none.
*a. Probability of a single arc intersection.*

1. The probability that the upper intersection point of the circles lies on the marked arc of the first circle, and the lower intersection point does not lie on this arc, is

$$\frac{2\beta(x)}{2\pi} = \frac{\beta(x)}{\pi}.$$

The probability that the upper point of the intersection of the circles lies on the marked arc of the second circle is

$$\frac{\varphi}{2\pi}.$$

The probability of simultaneous execution of these events is equal to

$$\frac{\varphi\beta(x)}{2\pi^2}.$$

2. The probability that the lower intersection point of the circles lies on the marked arc of the first circle, and the upper intersection point does not lie on this arc, is

$$\frac{2\beta(x)}{2\pi} = \frac{\beta(x)}{\pi}.$$

The probability that the lower point of the intersection of the circles lies on the marked arc of the second circle is

$$\frac{\varphi}{2\pi}.$$

The probability of simultaneous execution of these events is equal to

$$\frac{\varphi\beta(x)}{2\pi^2}.$$

3. The probability that both intersection points of the circles lie on the marked arc of the first circle is

$$\frac{\varphi - 2\beta(x)}{2\pi}.$$

The probability that the upper point of the intersection of the circles lies on the marked arc of the second circle and that the lower point of the intersection of the circles does not lie on the marked arc of the second circle is

$$\frac{2\beta(x)}{2\pi} = \frac{\beta(x)}{\pi}.$$

The probability of simultaneous execution of these events is equal to

$$\frac{[\varphi - 2\beta(x)]\beta(x)}{2\pi^2}.$$

4. The probability that the lower point of the intersection of the circles lies on the marked arc of the second circle and the upper point of the intersection of the circles does not lie on the marked arc of the second circle is

$$\frac{2\beta(x)}{2\pi} = \frac{\beta(x)}{\pi}.$$

The probability that this event occurs simultaneously and that both intersection points of the circles lie on the marked arc of the first circle is

$$\frac{[\varphi - 2\beta(x)]\beta(x)}{2\pi^2}.$$

The probability that the marked arcs have only one intersection point is

$$P^{(1)}(x) = 2\frac{\varphi\beta(x)}{2\pi^2} + 2\frac{[\varphi - 2\beta(x)]\beta(x)}{2\pi^2} = \frac{2\beta(x)[\varphi - \beta(x)]}{\pi^2}.$$

*b. The probability of intersecting arcs twice.* The probability that both intersection points of the circles lie on the marked arc of the first circle is

$$P_1^{(2)}(x) = \frac{\varphi - 2\beta(x)}{2\pi}.$$

The probability that both intersection points of the circles lie on the marked arc of the second circle is

$$P_2^{(2)}(x) = \frac{\varphi - 2\beta(x)}{2\pi}.$$

Since the locations of the arcs on the circles are independent and equally probable, the probability that both points of intersection of the circles belong to both labeled arcs is equal to

$$P^{(2)}(x) = P_1^{(2)}(x)P_2^{(2)}(x) = \left[\frac{\varphi - 2\beta(x)}{2\pi}\right]^2.$$

*c. The probability of intersecting arcs* is equal to

$$P(x) = P^{(1)}(x) + P^{(2)}(x) = \frac{2\beta(x)[\varphi - \beta(x)]}{\pi^2} + \left[\frac{\varphi - 2\beta(x)}{2\pi}\right]^2 = \frac{4\beta(x)\,[\varphi - \beta(x)] + \varphi^2}{4\pi^2}.$$

## III. PROBABILITIES OF INTERSECTING ARCS AT THE DISTANCE $x$ BETWEEN THE CENTERS OF THE CIRCLES

The probability that the arcs intersect only once is

$$P^{(1)}(x) = \begin{cases} \dfrac{\varphi^2}{2\pi^2}, & \text{if } \varphi < 2\beta(x), \\[2ex] \dfrac{2\beta(x)[\varphi - \beta(x)]}{\pi^2}, & \text{if } 2\beta(x) \leqslant \varphi \leqslant 2(\pi - \beta(x)), \\[2ex] \dfrac{4\varphi}{\pi} - \dfrac{3\varphi^2}{2\pi^2} - 2, & \text{if } \varphi > 2(\pi - \beta(x)). \end{cases}$$

The probability that the arcs intersect twice is

$$P^{(2)}(x) = \begin{cases} 0, & \text{if } \varphi < 2\beta(x), \\[2ex] \left[\dfrac{\varphi - 2\beta(x)}{2\pi}\right]^2, & \text{if } 2\beta(x) \leqslant \varphi \leqslant 2(\pi - \beta(x)), \\[2ex] \left(\dfrac{\varphi}{\pi} - 1\right)^2, & \text{if } \varphi > 2(\pi - \beta(x)). \end{cases}$$

The probability that the arcs intersect is

$$P(x) = \begin{cases} \dfrac{\varphi^2}{2\pi^2}, & \text{if } \varphi < 2\beta(x), \\[2ex] \dfrac{4\beta(x)\left[\varphi - \beta(x)\right] + \varphi^2}{4\pi^2}, & \text{if } 2\beta(x) \leqslant \varphi \leqslant 2(\pi - \beta(x)), \\[2ex] \dfrac{2\varphi}{\pi} - \dfrac{\varphi^2}{2\pi^2} - 1, & \text{if } \varphi > 2(\pi - \beta(x)). \end{cases}$$

## IV. ARBITRARY DISTANCE BETWEEN CIRCLE CENTERS

The probability that two arcs intersect is

$$P = \frac{1}{4\pi r^2} \int\limits_0^{2r} P(x) 2\pi x \, \mathrm{d}x.$$

If $\varphi < \pi$, then

$$P(\varphi) = \frac{1}{4\pi r^2} \int\limits_0^{2r\cos\frac{\varphi}{2}} \frac{\varphi^2}{2\pi^2} 2\pi x \, \mathrm{d}x + \frac{1}{4\pi r^2} \int\limits_{2r\cos\frac{\varphi}{2}}^{2r} \frac{4\beta(x)\left[\varphi - \beta(x)\right] + \varphi^2}{4\pi^2} 2\pi x \, \mathrm{d}x.$$

$$P(\varphi) = \frac{1}{8\pi^2}\left(3\varphi^2 - 2\cos\varphi + 2\right).$$

If the centers of the circles are uniformly randomly distributed in a region $L \times L$ with periodic boundary conditions, then the probability of the intersection of the two arcs will be

$$P^*(\varphi) = \frac{4\pi r^2}{L^2} P(\varphi).$$

$$\varphi = \frac{l}{r},$$

where $l$ is the arc length. If $r \to \infty$, then $\varphi \to 0$, $\sin\varphi \approx \varphi$, $\cos\varphi \approx 1 - \frac{\varphi^2}{2}$,

$$P(\varphi) \approx \frac{1}{2}\left(\frac{\varphi}{\pi}\right)^2.$$

$$P^*(\varphi) \approx \frac{4\pi r^2}{2L^2}\left(\frac{\varphi}{\pi}\right)^2 = \frac{2\pi r^2}{L^2}\left(\frac{l}{r\pi}\right)^2 = \frac{2l^2}{\pi L^2}.$$

$$P_{\text{stick}} \approx \frac{2l^2}{\pi L^2}.$$

*a. Comment.* In this limiting case (arcs of zero curvature, that is, segments), the obtained probability coincides with the value obtained for the rods.

In the limiting case, where $\varphi = \pi$,

$$P(\pi) = \frac{3}{8} + \frac{1}{2\pi^2}.$$

The probability that the arcs intersect at $\varphi \geqslant \pi$ is

$$P(\varphi) = \frac{1}{4\pi r^2}\int\limits_{-2r\cos\frac{\varphi}{2}}^{2r} \frac{4\beta(x)\left[\varphi - \beta(x)\right] + \varphi^2}{4\pi^2} 2\pi x\,\mathrm{d}x + \frac{1}{4\pi r^2}\int\limits_{0}^{-2r\cos\frac{\varphi}{2}} \left(\frac{2\varphi}{\pi} - \frac{\varphi^2}{2\pi^2} - 1\right) 2\pi x\,\mathrm{d}x.$$

$$P(\varphi) = \frac{1}{8\pi^2}\left[4(\pi - \varphi)\sin\varphi - 2\cos\varphi - 4\pi^2 + 8\varphi\pi - \varphi^2 + 2\right].$$

In the limiting case, where $\varphi = \pi$,

$$P(\pi) = \frac{3}{8} + \frac{1}{2\pi^2}.$$

In the limiting case, where $\varphi = 2\pi$,

$$P(2\pi) = 1.$$

Combining both cases, we have

$$P(\varphi) = \frac{1}{8\pi^2}\begin{cases} 3\varphi^2 - 2\cos\varphi + 2, & \text{if } \varphi < \pi, \\ 4(\pi - \varphi)\sin\varphi - 2\cos\varphi - 4\pi^2 + 8\varphi\pi - \varphi^2 + 2, & \text{if } \pi \geqslant \varphi. \end{cases}$$

If $\varphi < \pi$, then the probability that the arcs intersect twice is

$$P^{(2)}(\varphi) = \frac{1}{4\pi r^2}\int\limits_{2r\cos\frac{\varphi}{2}}^{2r} \left[\frac{\varphi - 2\beta(x)}{2\pi}\right]^2 2\pi x\,\mathrm{d}x = \frac{1}{8\pi^2 r^2}\int\limits_{2r\cos\frac{\varphi}{2}}^{2r} \left[\varphi - 2\arccos\frac{x}{2r}\right]^2 x\,\mathrm{d}x$$

$$P^{(2)}(\varphi) = \frac{1}{8\pi^2}\left[\varphi^2 - 2 + 2\cos\varphi\right].$$

In the limiting case, where $\varphi = \pi$,

$$P^{(2)}(\pi) = \frac{1}{8} - \frac{1}{2\pi^2}.$$

If $\varphi \geqslant \pi$, then the probability that the arcs intersect twice is

$$P^{(2)}(\varphi) = \frac{1}{4\pi r^2} \int\limits_0^{-2r\cos\frac{\varphi}{2}} \left(\frac{\varphi}{\pi} - 1\right)^2 2\pi x \, \mathrm{d}x + \frac{1}{4\pi r^2} \int\limits_{-2r\cos\frac{\varphi}{2}}^{2r} \left[\frac{\varphi - 2\beta(x)}{2\pi}\right]^2 2\pi x \, \mathrm{d}x,$$

$$P^{(2)}(\varphi) = \frac{1}{8\pi^2}\left(-4\pi\sin\varphi + 4\varphi\sin\varphi + 2\cos\varphi - 2 + 4\pi^2 - 8\pi\varphi + 5\varphi^2\right).$$

In the limiting case, where $\varphi = \pi$,

$$P^{(2)}(\pi) = \frac{1}{8} - \frac{1}{2\pi^2}.$$

In the limiting case, where $\varphi = 2\pi$,

$$P^{(2)}(2\pi) = 1.$$

Combining both cases $\varphi < \pi$ and $\varphi \geqslant \pi$, we have

$$P^{(2)}(\varphi) = \begin{cases} \frac{1}{8\pi^2}\left(\varphi^2 - 2 + 2\cos\varphi\right), & \text{if } \varphi < \pi, \\ \frac{1}{8\pi^2}\left(-4\pi\sin\varphi + 4\varphi\sin\varphi + 2\cos\varphi - 2 + 4\pi^2 - 8\pi\varphi + 5\varphi^2\right), & \text{if } \varphi \geqslant \pi. \end{cases}$$

The probability that the arcs intersect once at $\varphi < \pi$ is equal to

$$P^{(1)}(\varphi) = \frac{1}{4\pi r^2} \int\limits_0^{2r\cos\frac{\varphi}{2}} \frac{\varphi^2}{2\pi^2} 2\pi x \, \mathrm{d}x + \frac{1}{4\pi r^2} \int\limits_{2r\cos\frac{\varphi}{2}}^{2r} \frac{2\beta(x)[\varphi - \beta(x)]}{\pi^2} 2\pi x \, \mathrm{d}x.$$

$$P^{(1)}(\varphi) = \frac{1}{4\pi^2}\left(\varphi^2 - 2\cos\varphi + 2\right).$$

In the limiting case, where $\varphi = \pi$,

$$P^{(1)}(\pi) = \frac{1}{4} + \frac{1}{\pi^2}.$$

The probability that the arcs intersect once at $\varphi \geqslant \pi$ is equal to

$$P^{(1)}(\varphi) = \frac{1}{4\pi r^2} \int\limits_0^{-2r\cos\frac{\varphi}{2}} \left(\frac{4\varphi}{\pi} - \frac{3\varphi^2}{2\pi^2} - 2\right) 2\pi x \, \mathrm{d}x + \frac{1}{4\pi r^2} \int\limits_{-2r\cos\frac{\varphi}{2}}^{2r} \frac{2\beta(x)[\varphi - \beta(x)]}{\pi^2} 2\pi x \, \mathrm{d}x,$$

$$P^{(1)}(\varphi) = \frac{1}{4\pi^2}\left[4\pi\sin\varphi - 4\varphi\sin\varphi - 2\cos\varphi + 2 - 4\pi^2 + 8\pi\varphi - 3\varphi^2\right].$$

In the limiting case, where $\varphi = \pi$,

$$P^{(1)}(\pi) = \frac{1}{4} + \frac{1}{\pi^2}.$$

In the limiting case, where $\varphi = 2\pi$,

$$P^{(1)}(2\pi) = 0.$$

Combining both cases $\varphi < \pi$ and $\varphi \geqslant \pi$, we have

$$P^{(1)}(\varphi) = \frac{1}{4\pi^2} \begin{cases} \varphi^2 - 2\cos\varphi + 2, & \text{if } \varphi < \pi \\ 4(\pi - \varphi)\sin\varphi - 2\cos\varphi - 4\pi^2 + 8\pi\varphi + 2 - 3\varphi^2, & \text{if } \varphi \geqslant \pi. \end{cases}$$

*b. All formulas together.*

$$P^{(1)}(\varphi) = \frac{1}{4\pi^2}\begin{cases} \varphi^2 - 2\cos\varphi + 2, & \text{if } \varphi < \pi \\ 4(\pi-\varphi)\sin\varphi - 2\cos\varphi - 4\pi^2 + 8\pi\varphi + 2 - 3\varphi^2, & \text{if } \varphi \geqslant \pi. \end{cases}$$

$$P^{(2)}(\varphi) = \frac{1}{8\pi^2}\begin{cases} \varphi^2 + 2\cos\varphi - 2, & \text{if } \varphi < \pi, \\ -4(\pi-\varphi)\sin\varphi + 2\cos\varphi + 4\pi^2 - 8\pi\varphi - 2 + 5\varphi^2, & \text{if } \varphi \geqslant \pi. \end{cases}$$

$$P(\varphi) = \frac{1}{8\pi^2}\begin{cases} 3\varphi^2 - 2\cos\varphi + 2, & \text{if } \varphi < \pi, \\ 4(\pi-\varphi)\sin\varphi - 2\cos\varphi - 4\pi^2 + 8\varphi\pi + 2 - \varphi^2, & \text{if } \pi \geqslant \varphi. \end{cases}$$

## V. AVERAGE NUMBER OF CONTACTS PER ARC

Let there be $N$ circles of radius $r$. The centers of the circles are uniformly randomly distributed in the region $L \times L$ with periodic boundary conditions, and the orientations of the arcs are equiprobable. Two circles intersect if the distance between their centroids does not exceed 2r. The probability that two circles intersect is

$$P_0 = \frac{4\pi r^2}{L^2}.$$

The number of intersections of the circles obeys a binomial distribution.

$$\Pr(N_{\text{ring}} = m) = C_N^m P_0^m (1-P_0)^{N-m-1}.$$

Expected value of the number of intersections of the circles is

$$\langle m \rangle = P_0(N-1) \approx NP_0.$$

$$\langle m \rangle \approx N\frac{4\pi r^2}{L^2} = 4\pi r^2 n.$$

Consequently, the average number of intersecting arcs is

$$\langle m \rangle P(\varphi) = 4\pi r^2 n P(\varphi).$$

The average number of contacts of intersecting arcs is

$$\langle k \rangle = 1 + \frac{P^{(2)}(\varphi)}{P(\varphi)}.$$

$$\langle k(\varphi) \rangle = 1 + \begin{cases} \dfrac{\varphi^2 - 2 + 2\cos\varphi}{3\varphi^2 - 2\cos\varphi + 2}, & \text{if } \varphi < \pi, \\ \dfrac{-4\pi\sin\varphi + 4\varphi\sin\varphi + 2\cos\varphi - 2 + 4\pi^2 - 8\pi\varphi + 5\varphi^2}{4(\pi-\varphi)\sin\varphi - 2\cos\varphi - 4\pi^2 + 8\varphi\pi - \varphi^2 + 2}, & \text{if } \varphi \geqslant \pi. \end{cases}$$

Comparison of the obtained formula with the simulation results is shown in Figs. 2.

Since

$$P(\varphi) + P^{(2)}(\varphi) = \frac{\varphi^2}{2\pi^2},$$

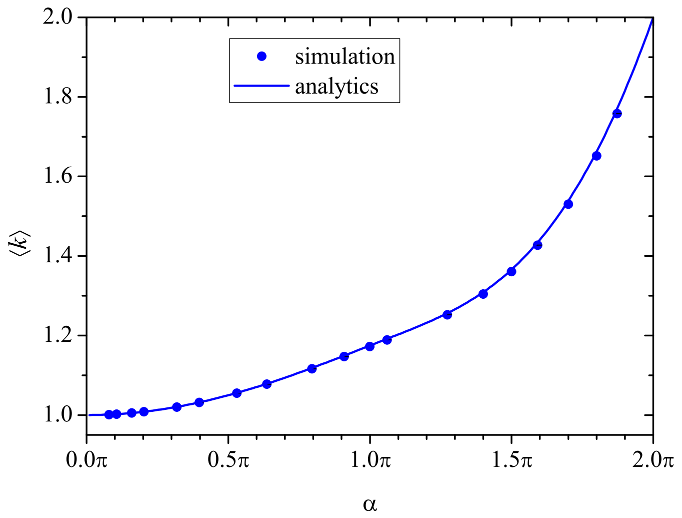


FIG. 2. Dependence of the average number of contacts between two identical intersecting arcs on the angular size of the arc.

then the average number of contacts per arc is

$$4\pi r^2 n P(\varphi)\langle k\rangle = 4\pi r^2 n \left[P(\varphi) + P^{(2)}(\varphi)\right] = \frac{2nl^2}{\pi},$$

where $l$ is the arc length. The resulting expression coincides with the average number of contacts in the case of rods of zero thickness and length $l$, which is in full agreement with the idea presented in the paper [1].

If the resistance of one contact is $R_\mathrm{j}$, then the average conductivity of the contacts per unit length is

$$G = \frac{4\pi r^2 n \left[P(\varphi) + P^{(2)}(\varphi)\right]}{\varphi r R_\mathrm{j}},$$

whence

$$G = \frac{2rn\varphi}{\pi R_\mathrm{j}} = \frac{2ln}{\pi R_\mathrm{j}}.$$

Written in terms of the arc length, the leakage electrical conductivity per unit length coincides with the formula obtained for rods of length $l$ [2].

$$\lambda^2 = r^2 \rho_\mathrm{w} G = \frac{2\varphi n r^3 \rho_\mathrm{w}}{\pi R_\mathrm{j}} = \frac{2nl^3\rho_\mathrm{w}}{\pi \varphi^2 R_\mathrm{j}}.$$

[1] Y. B. Yi, L. Berhan, and A. M. Sastry, Statistical geometry of random fibrous networks, revisited: Waviness, dimensionality, and percolation, J. Appl. Phys. **96**, 1318 (2004).
[2] Y. Y. Tarasevich, A. V. Eserkepov, and I. V. Vodolazskaya, Electrical conductivity of nanorod-based transparent electrodes: Comparison of mean-field approaches, Phys. Rev. E **105**, 044129 (2022).
